# Supplementary material for: ScanNet++: A High-Fidelity Dataset of 3D Indoor Scenes
Source: arXiv:2308.11417 source file (2023-08-22)
Supplement: Supplementary file 1 [file supplemental.tex]

\documentclass[10pt,twocolumn,letterpaper]{article}

\usepackage{iccv}
\usepackage{times}
\usepackage{epsfig}
\usepackage{graphicx}
\usepackage{amsmath}
\usepackage{amssymb}
\usepackage{subcaption}
\usepackage{booktabs}
\usepackage[dvipsnames]{xcolor}
\usepackage{multirow}
\usepackage{pifont}% http://ctan.org/pkg/pifont
\usepackage{comment}
\usepackage{caption}
\usepackage{floatpag}

\usepackage[pagebackref=true,breaklinks=true,letterpaper=true,colorlinks,bookmarks=false]{hyperref}

\iccvfinalcopy

\newcommand{\OURS}{ScanNet++}
\newcommand{\datasetname}{\OURS}

\begin{document}

%%%%%%%%% TITLE
\title{\datasetname: A High-Fidelity Dataset of 3D Indoor Scenes \\ [1ex]
\large Supplementary Material }

\maketitle

\input{arxiv/06_appendix}

{\small
\bibliographystyle{ieee_fullname}
\bibliography{egbib}
}
\end{document}
